# Supplementary material for: The JCMT Gould Belt Survey: A First Look at the Auriga-California Molecular Cloud with SCUBA-2
Source: arXiv:1801.08139 source file (2018-01-24)
Supplement: Supplementary file 1 [file appendix_figure.pdf]

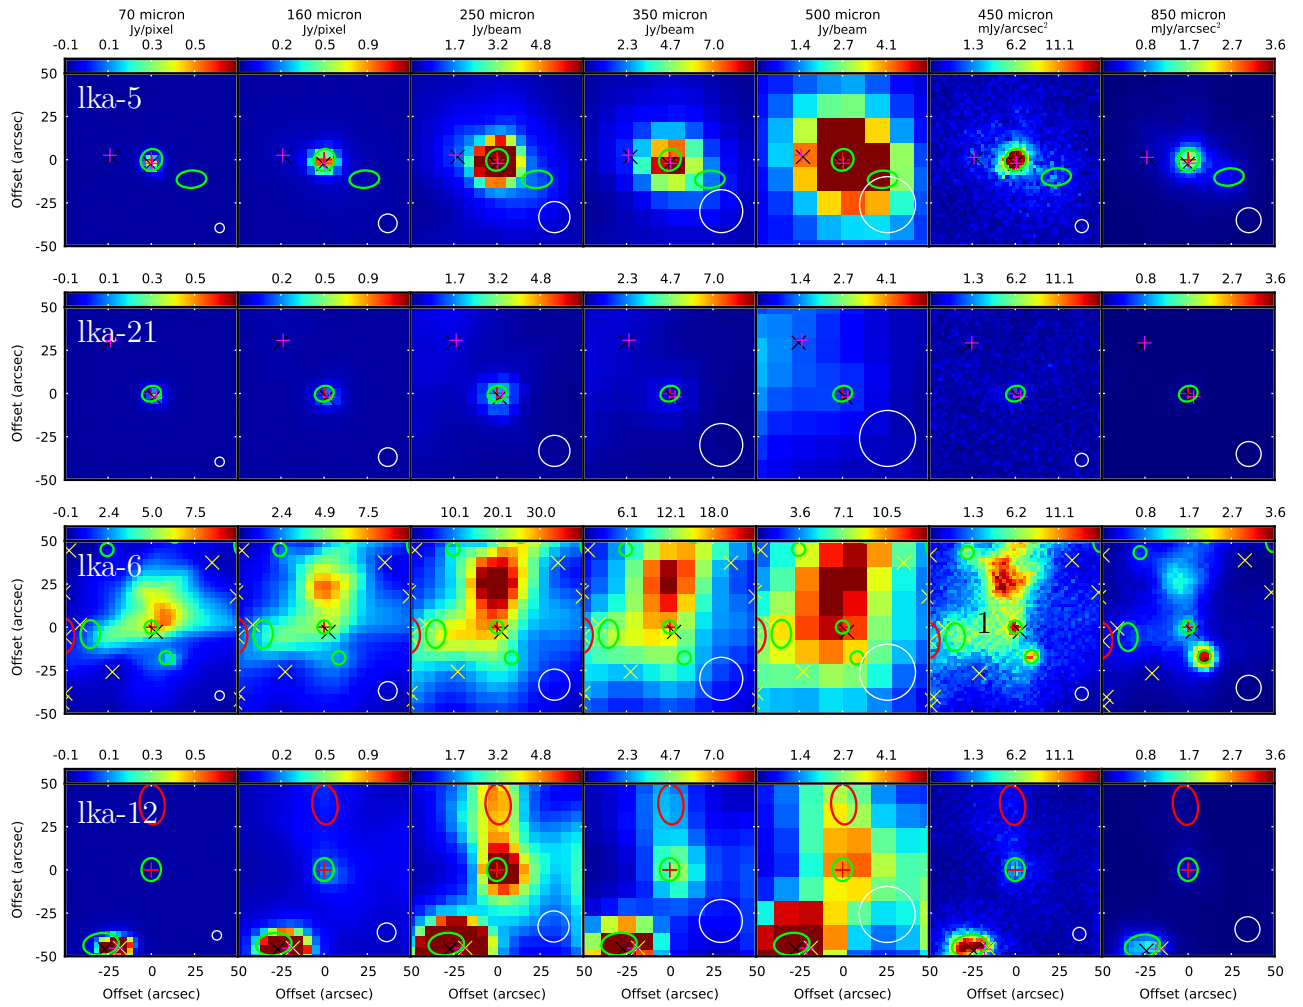

Figure 1:

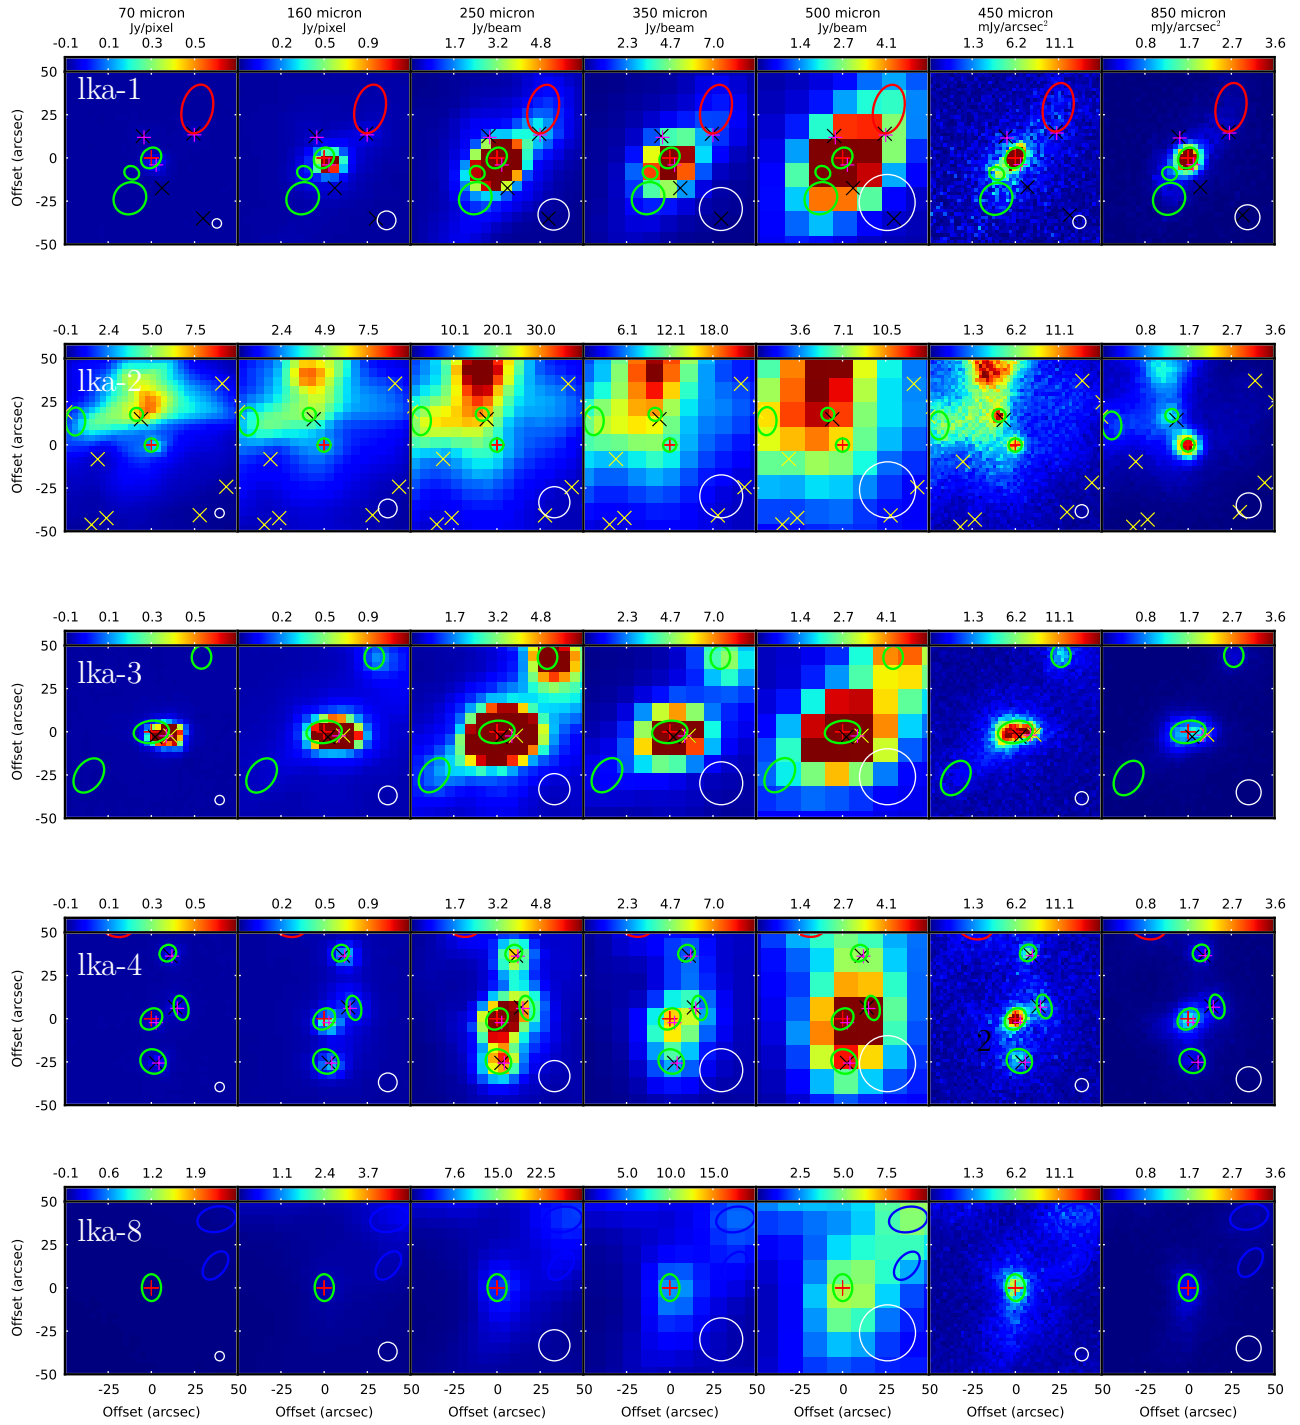

Figure 2:

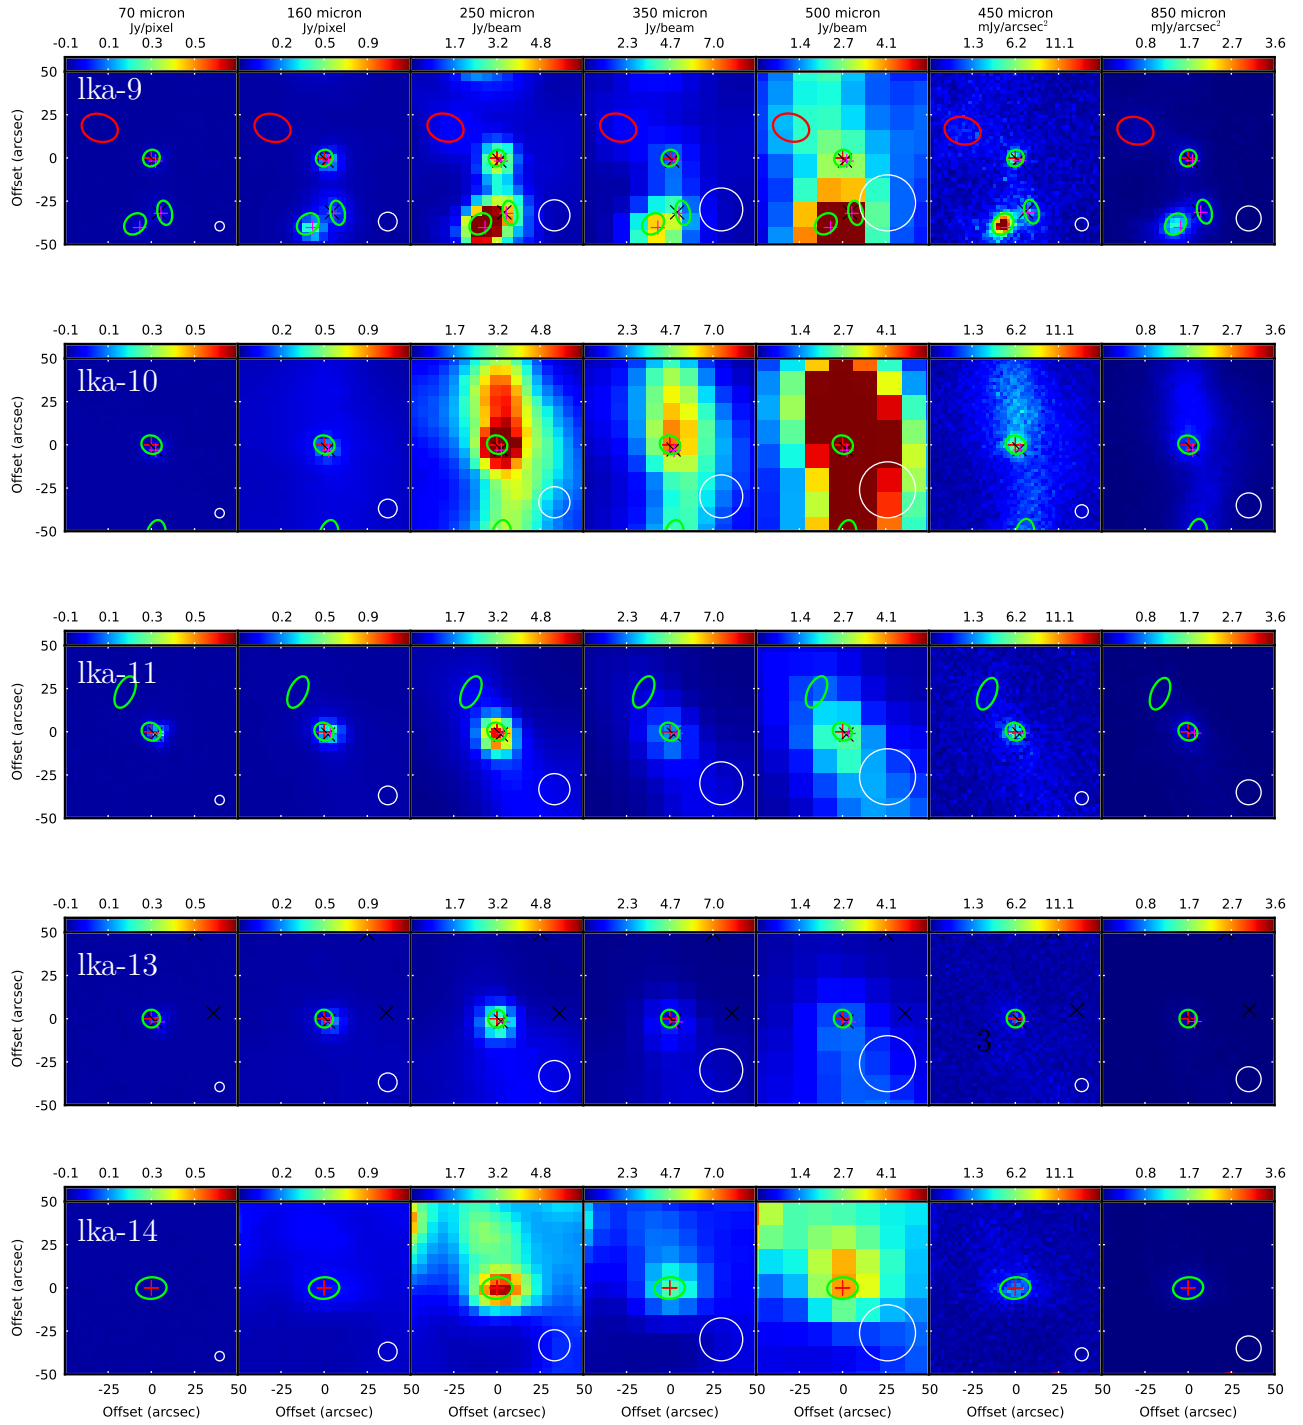

Figure 3:

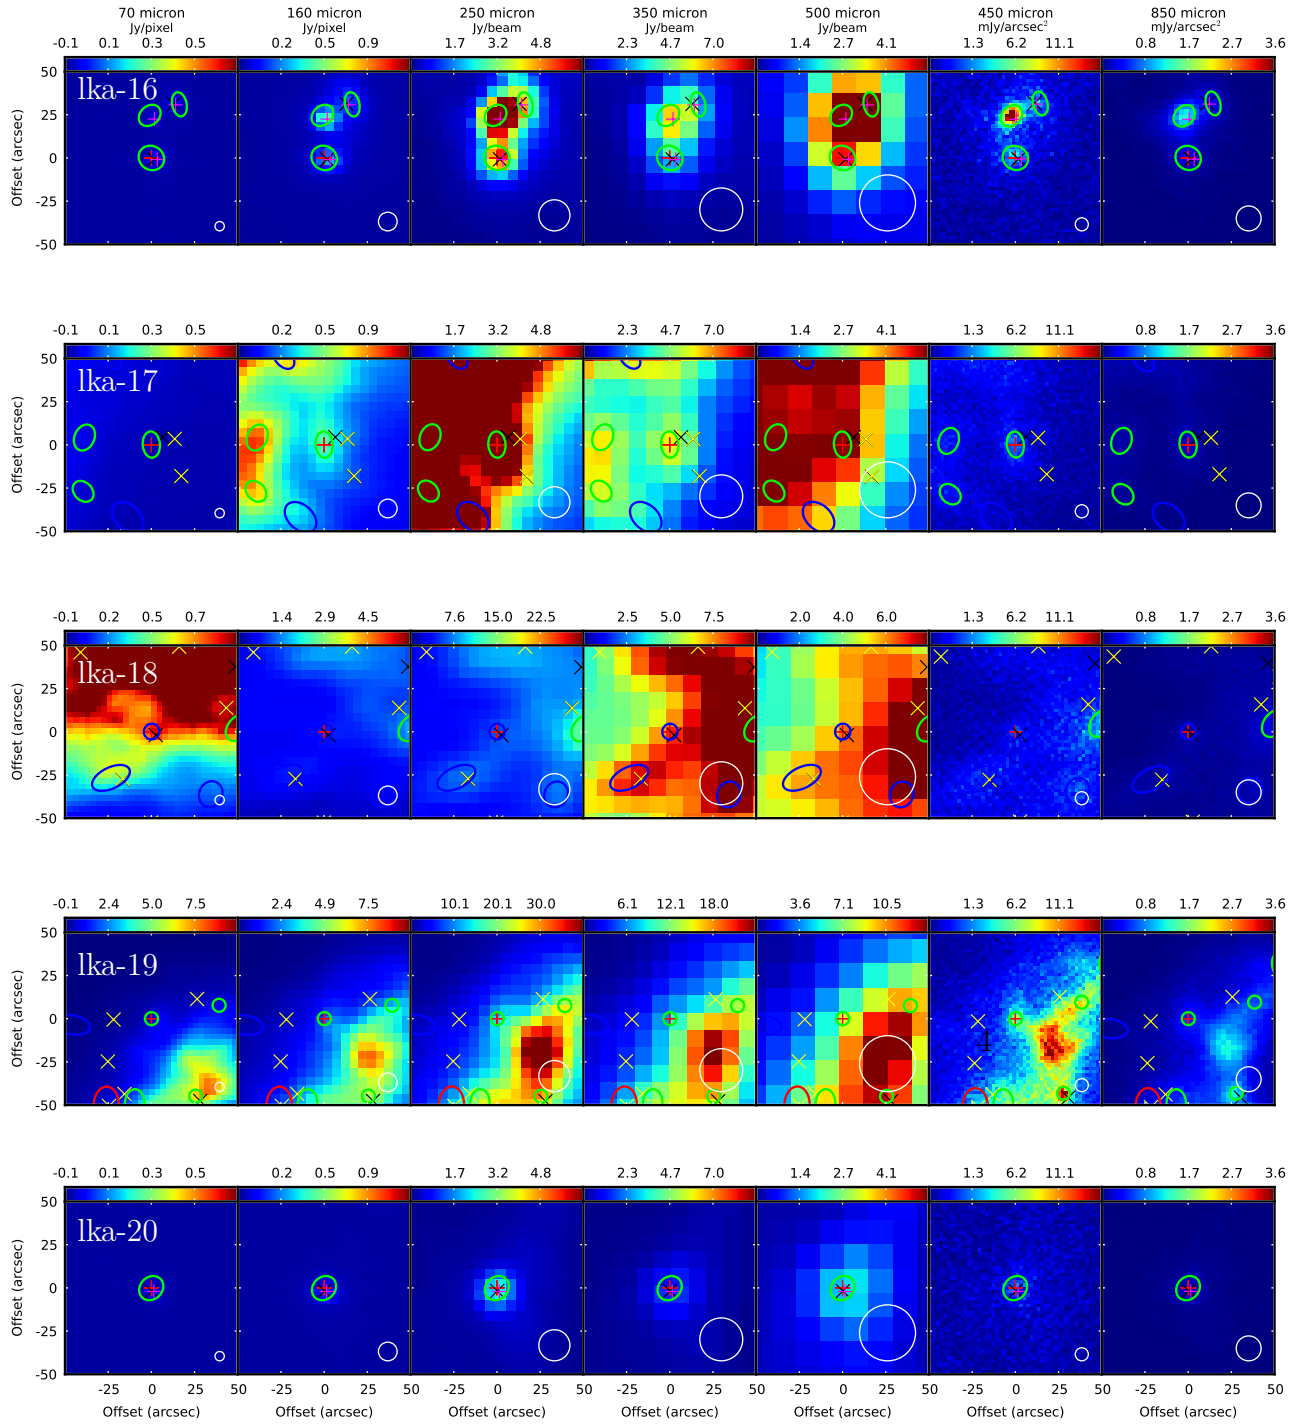

Figure 4:

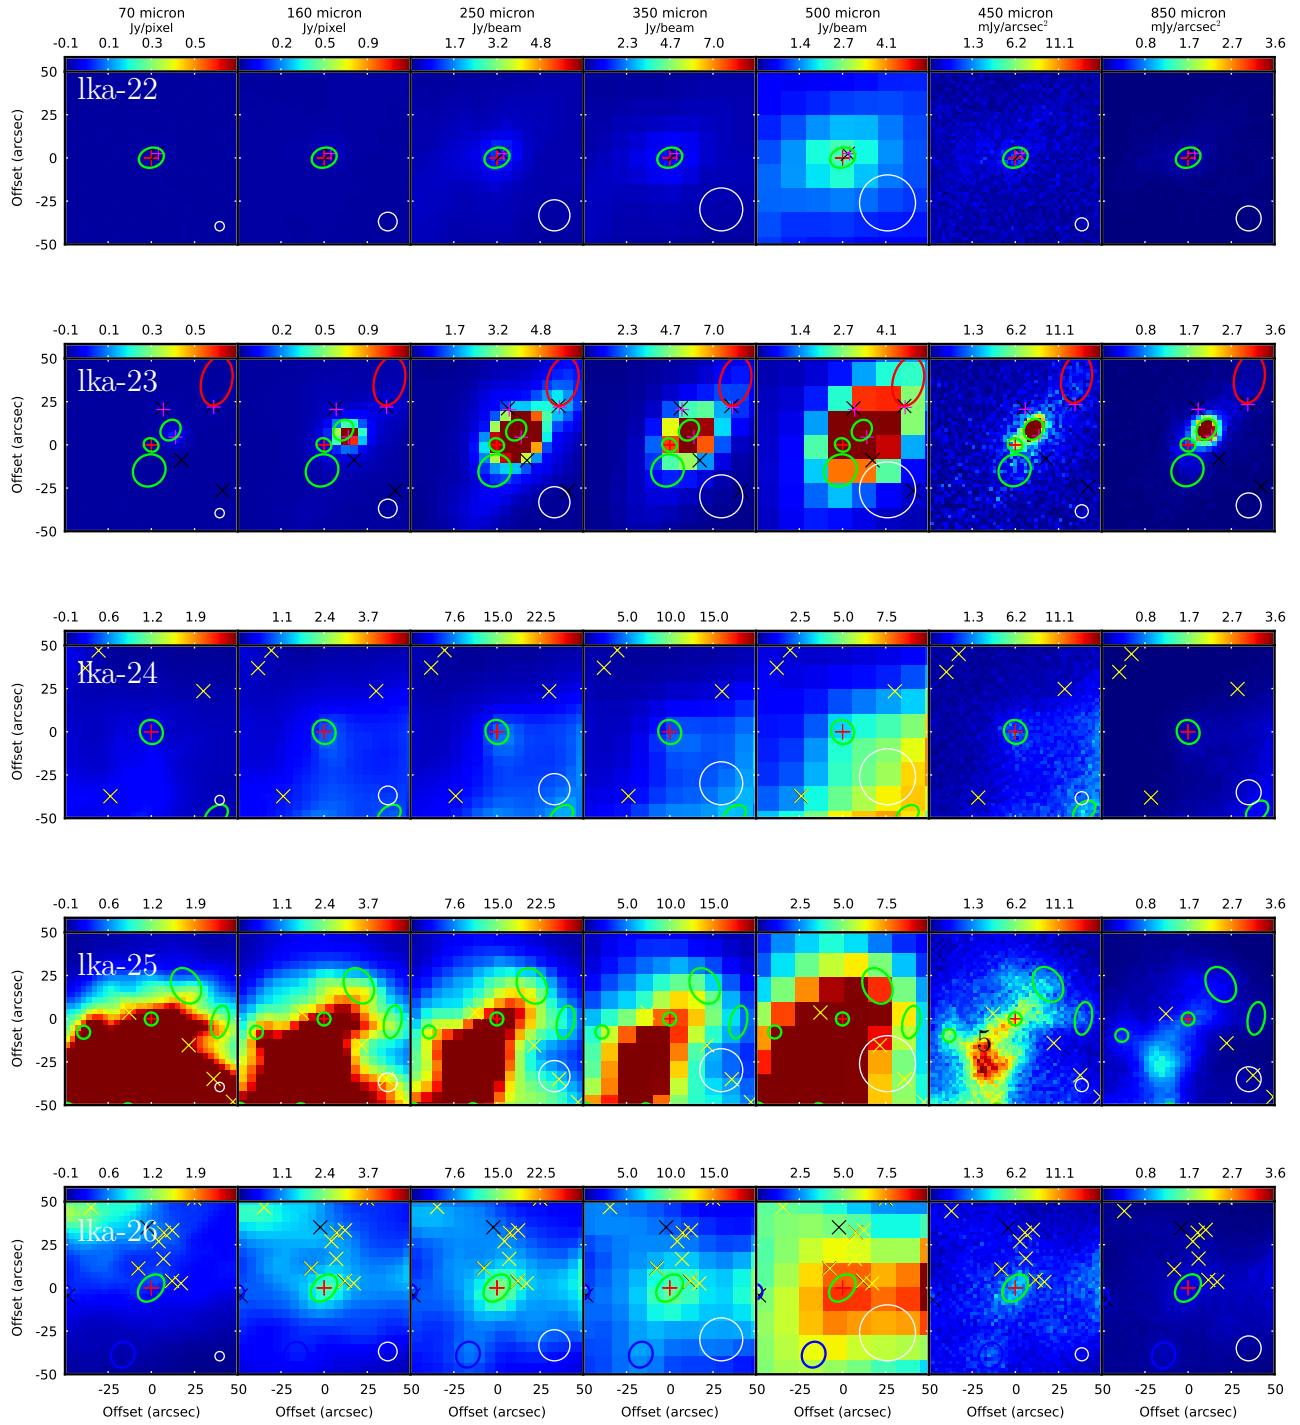

Figure 5:

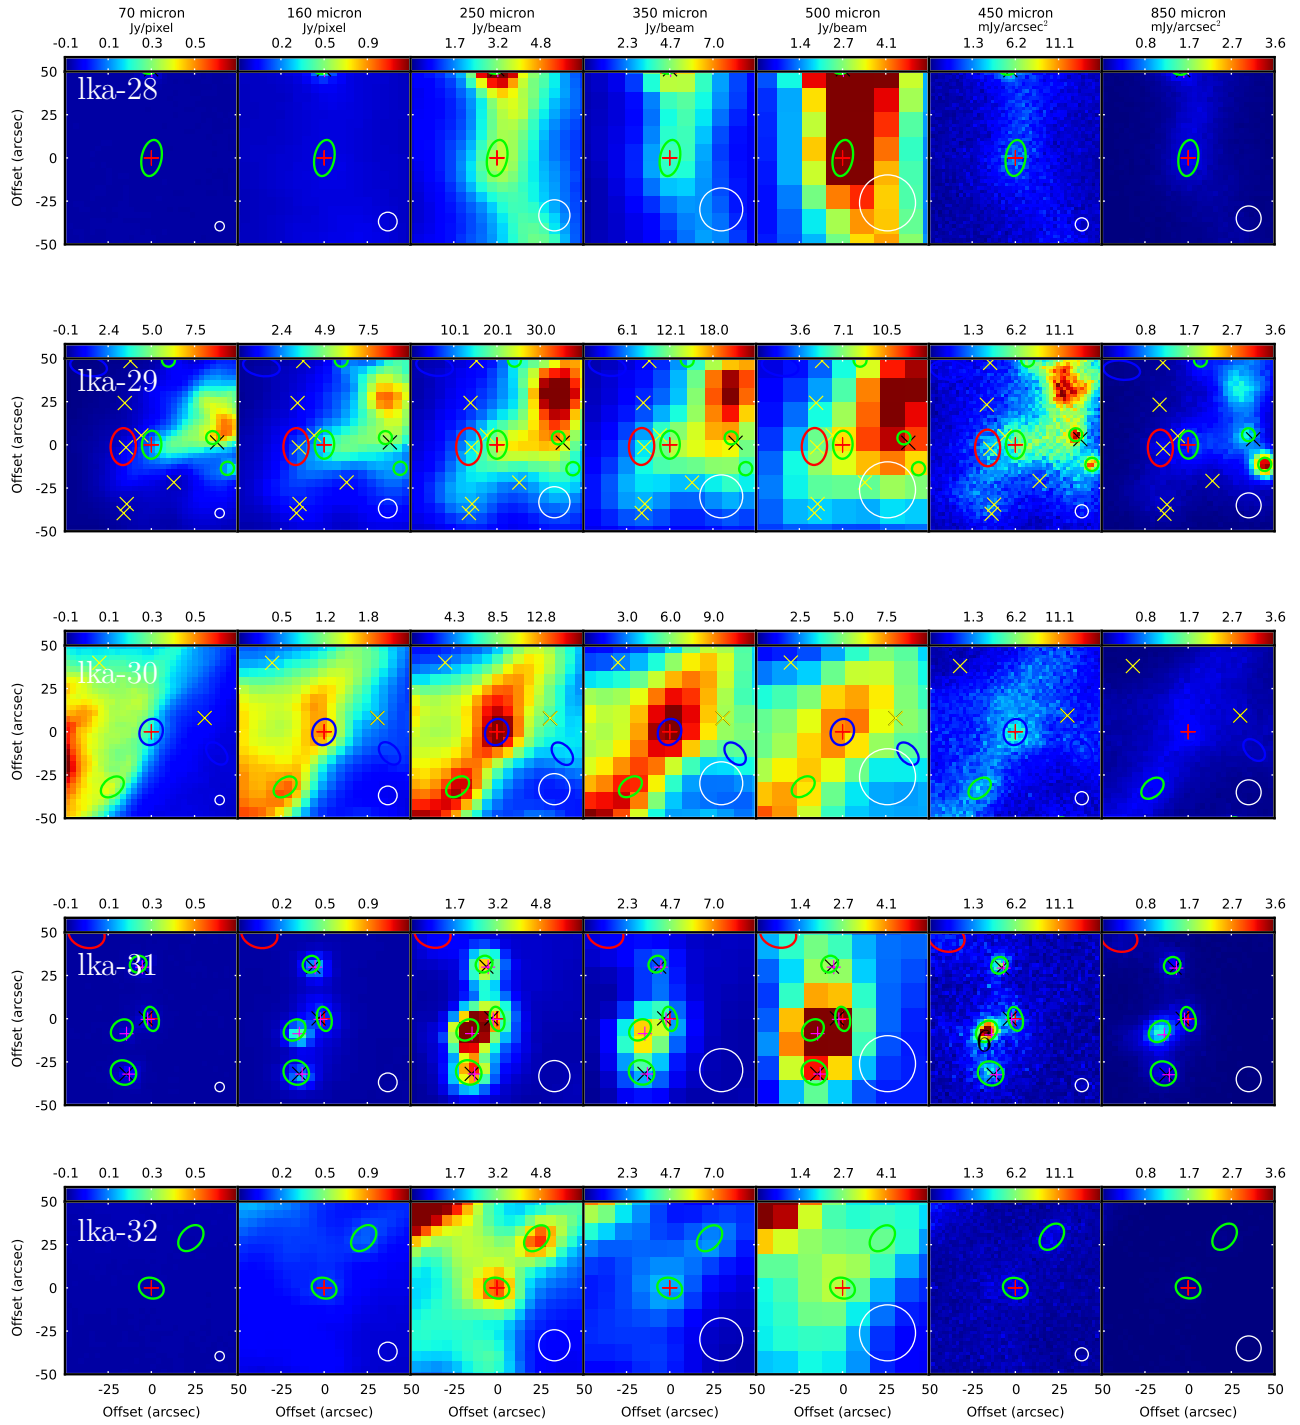

Figure 6:

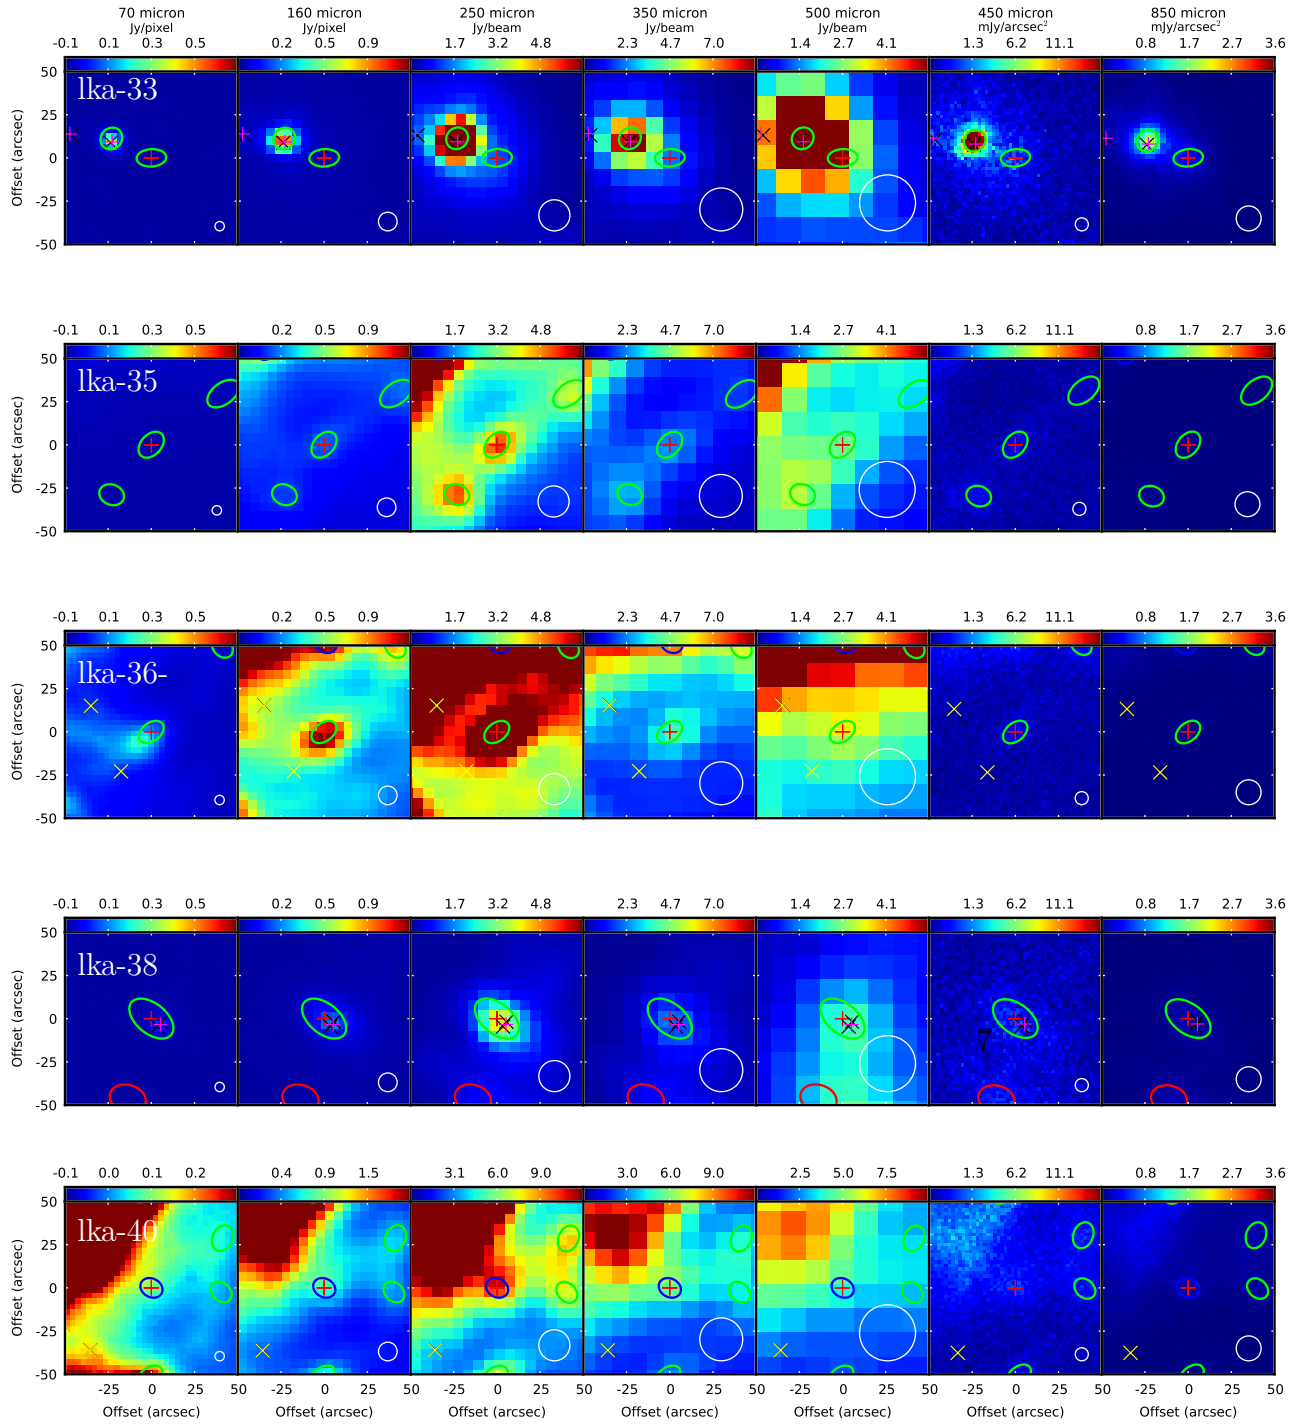

Figure 7:

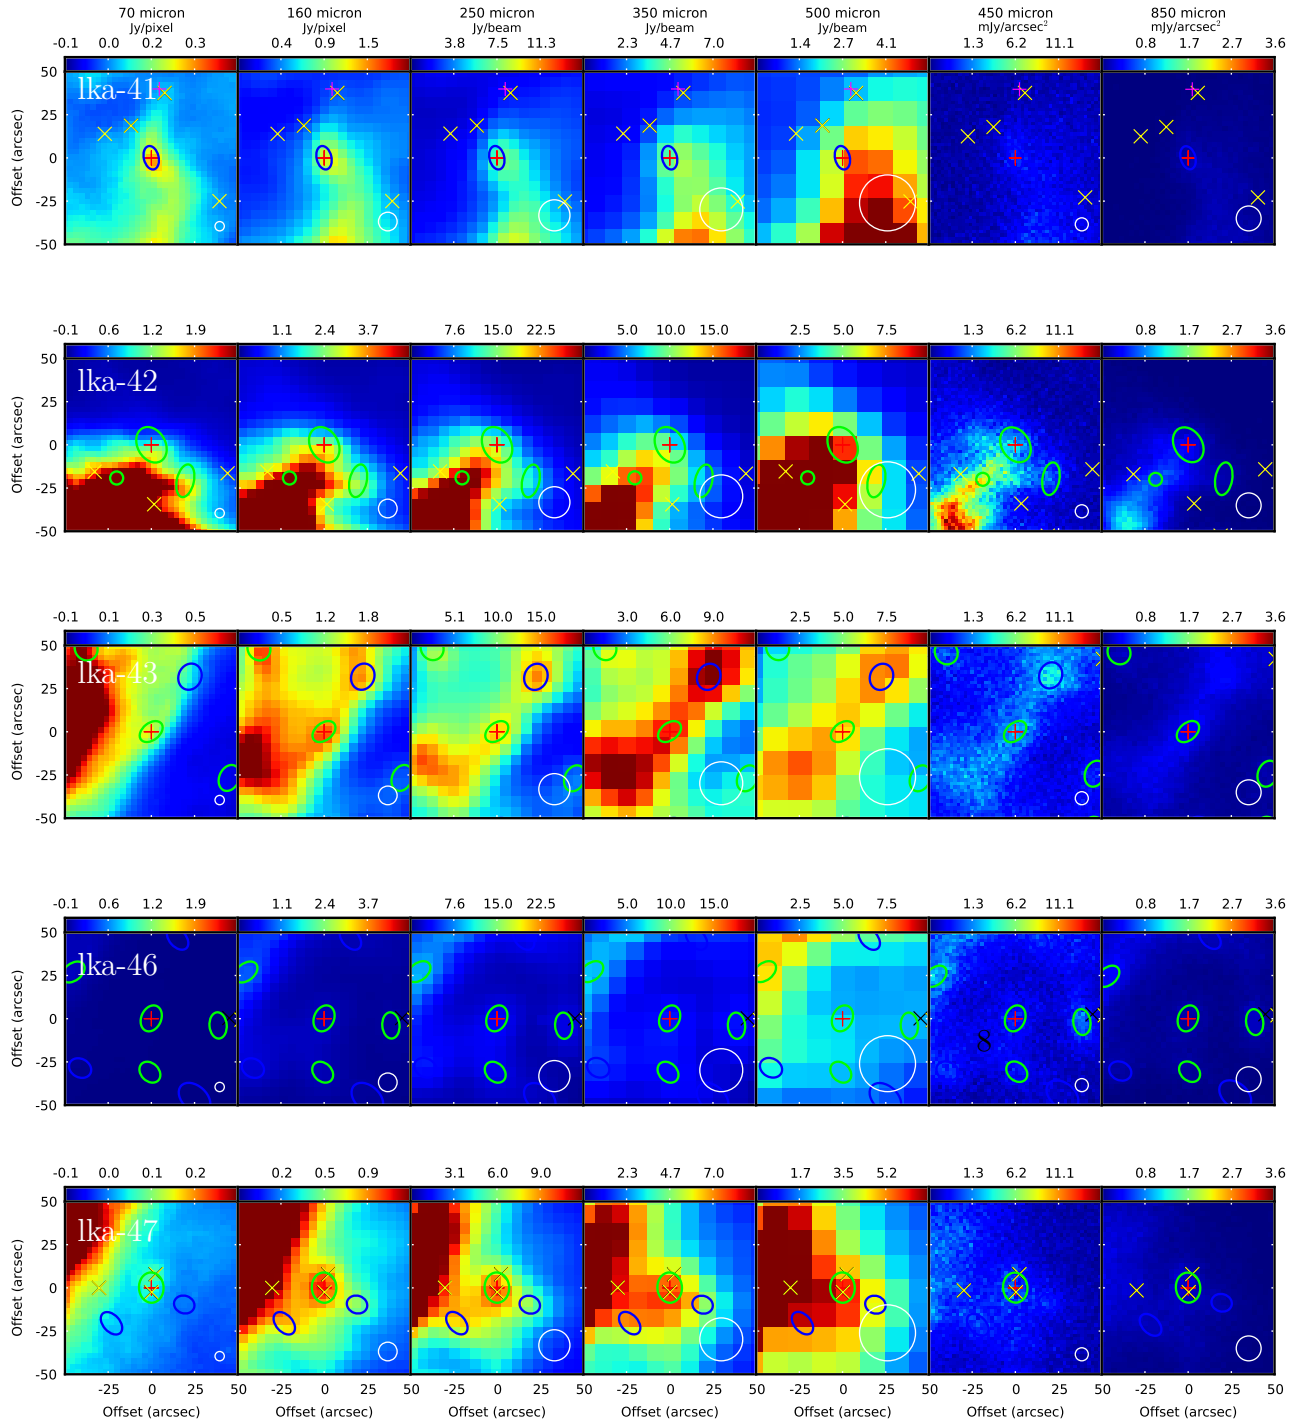

Figure 8:



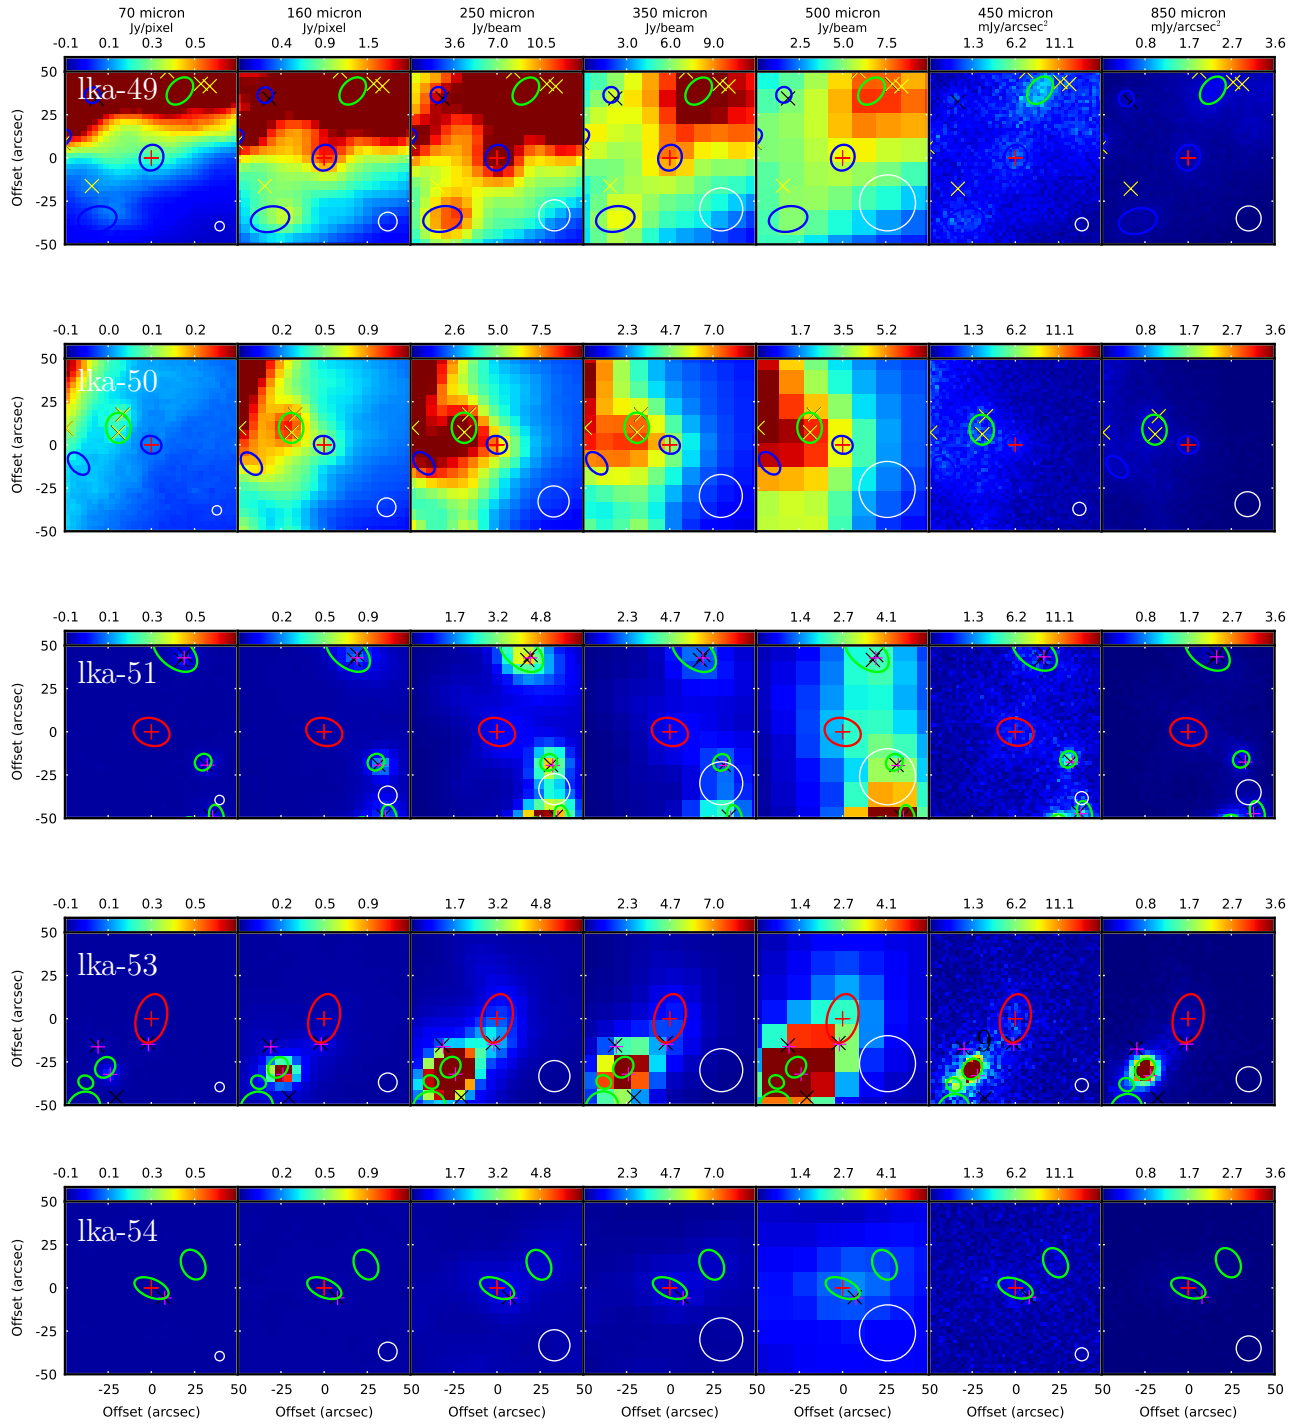

Figure 9:

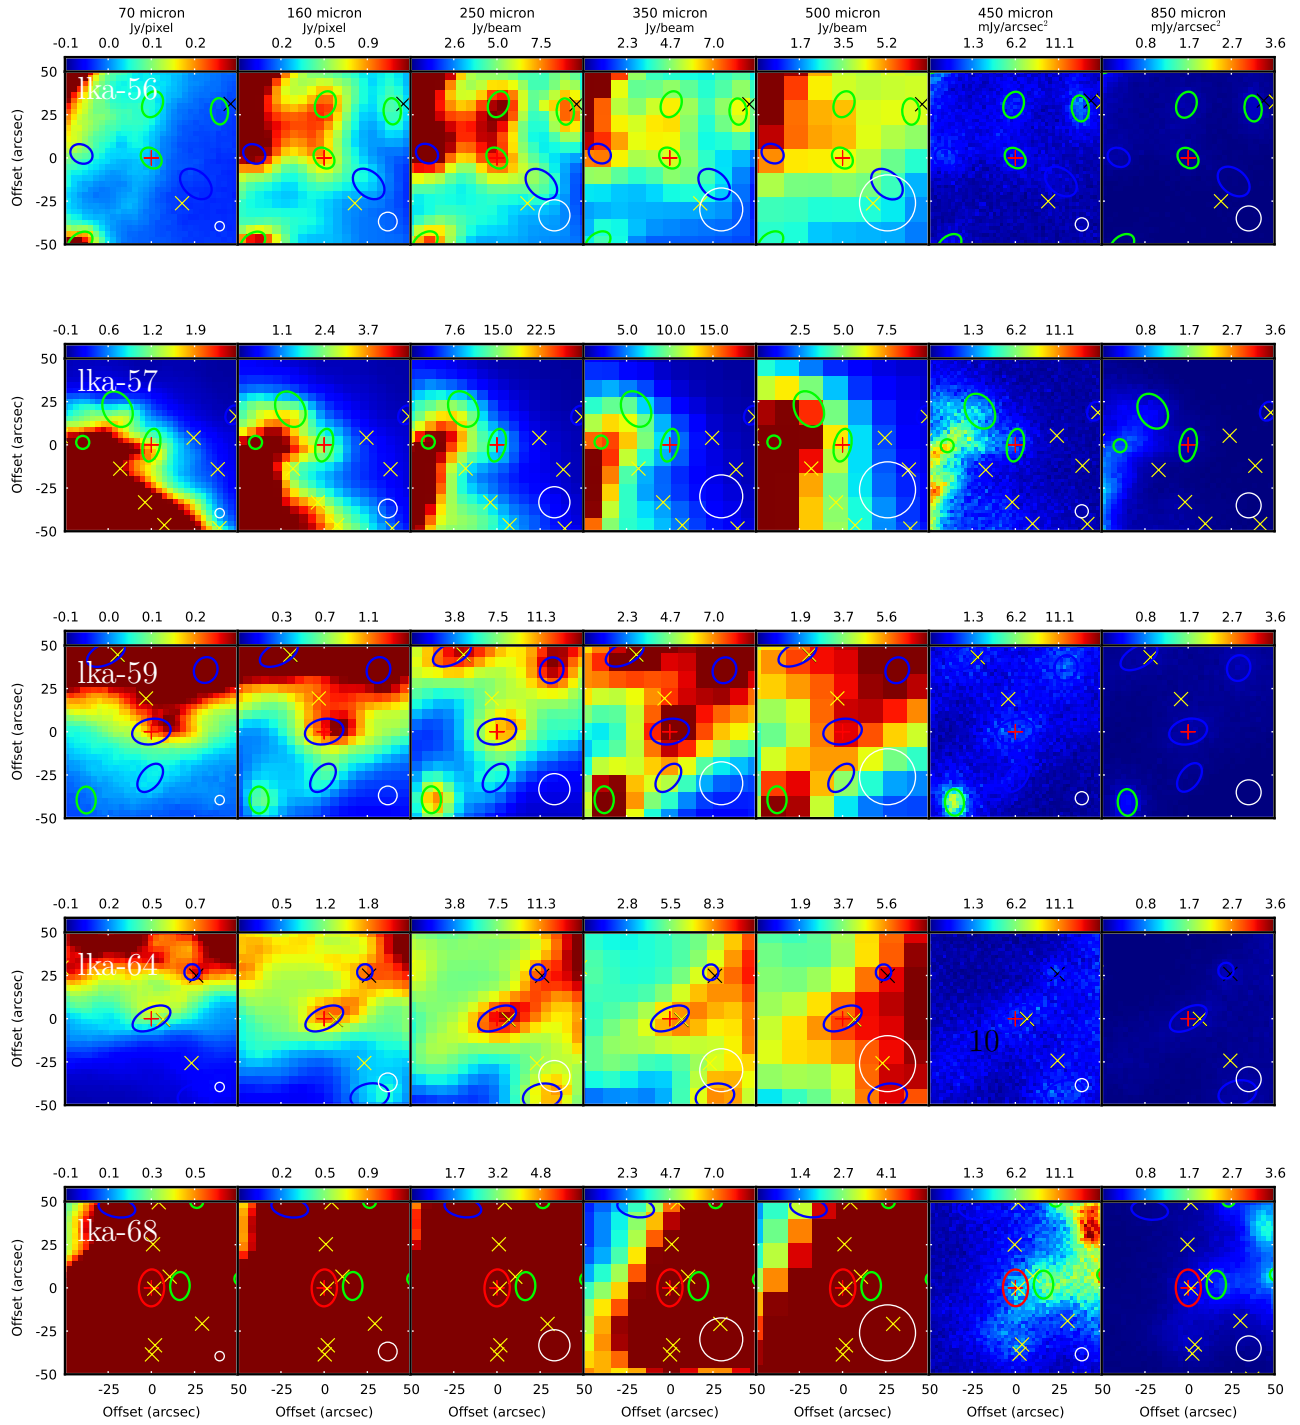

Figure 10:

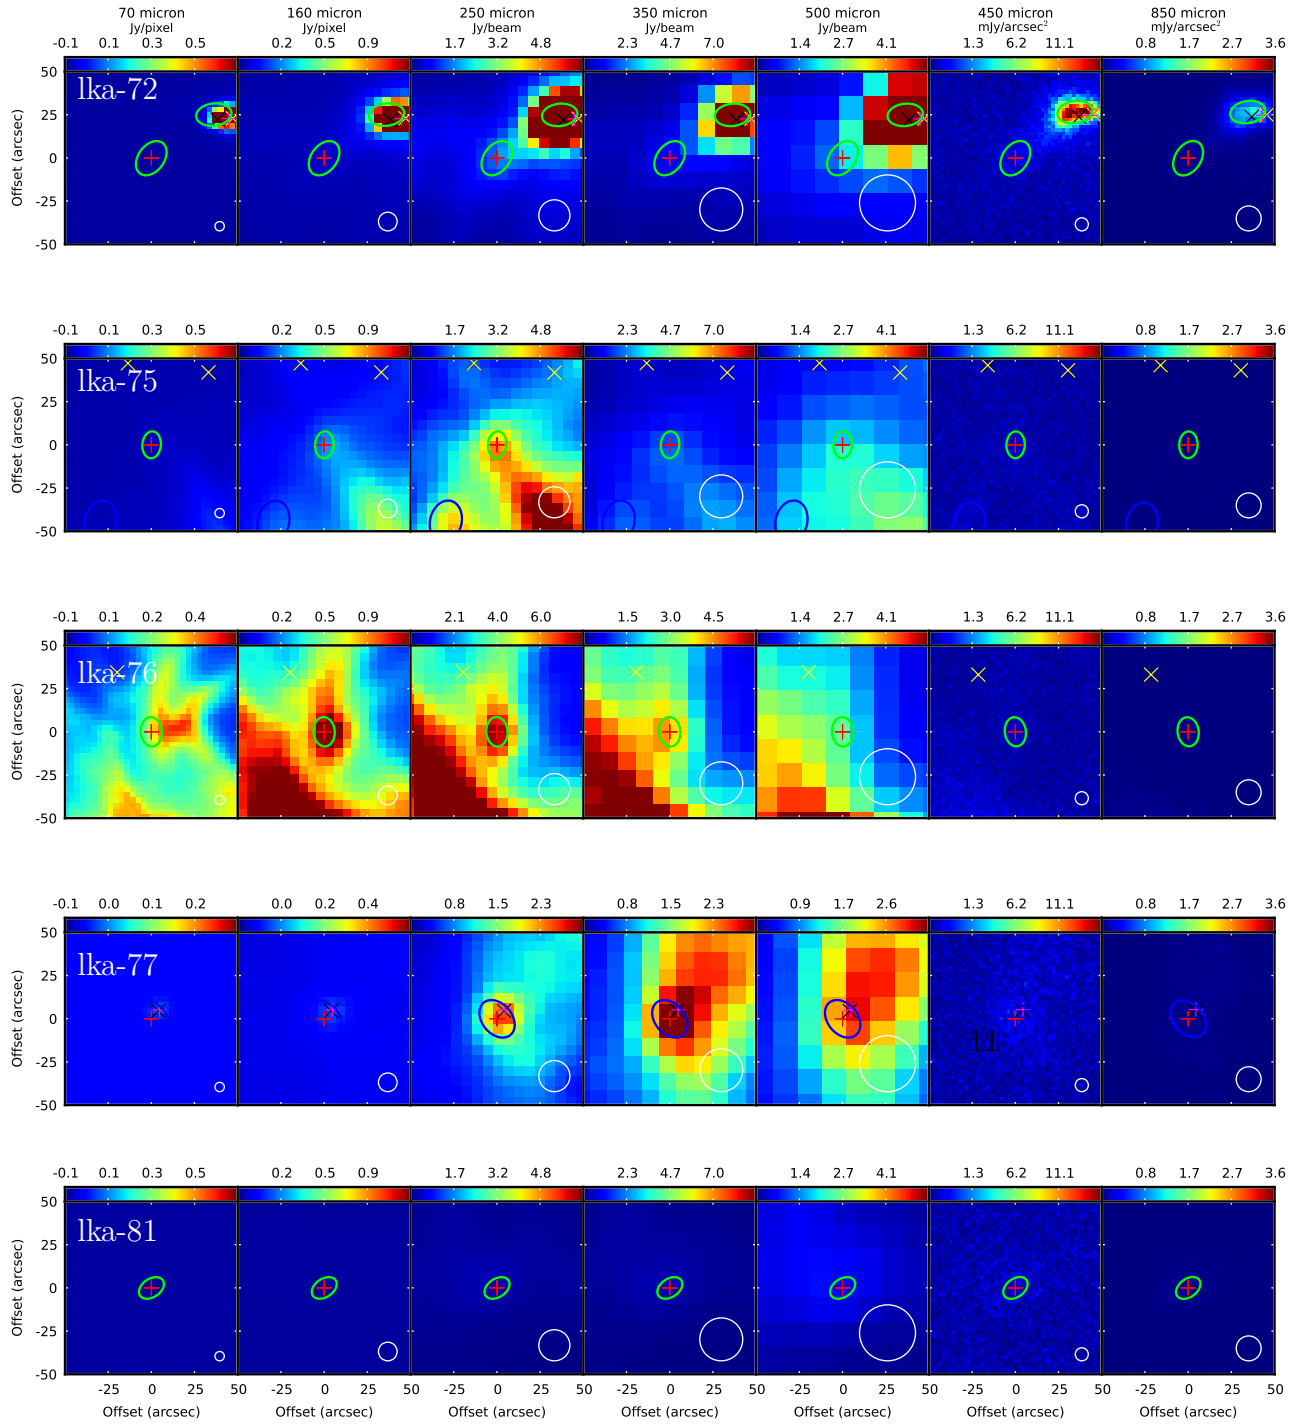

Figure 11:

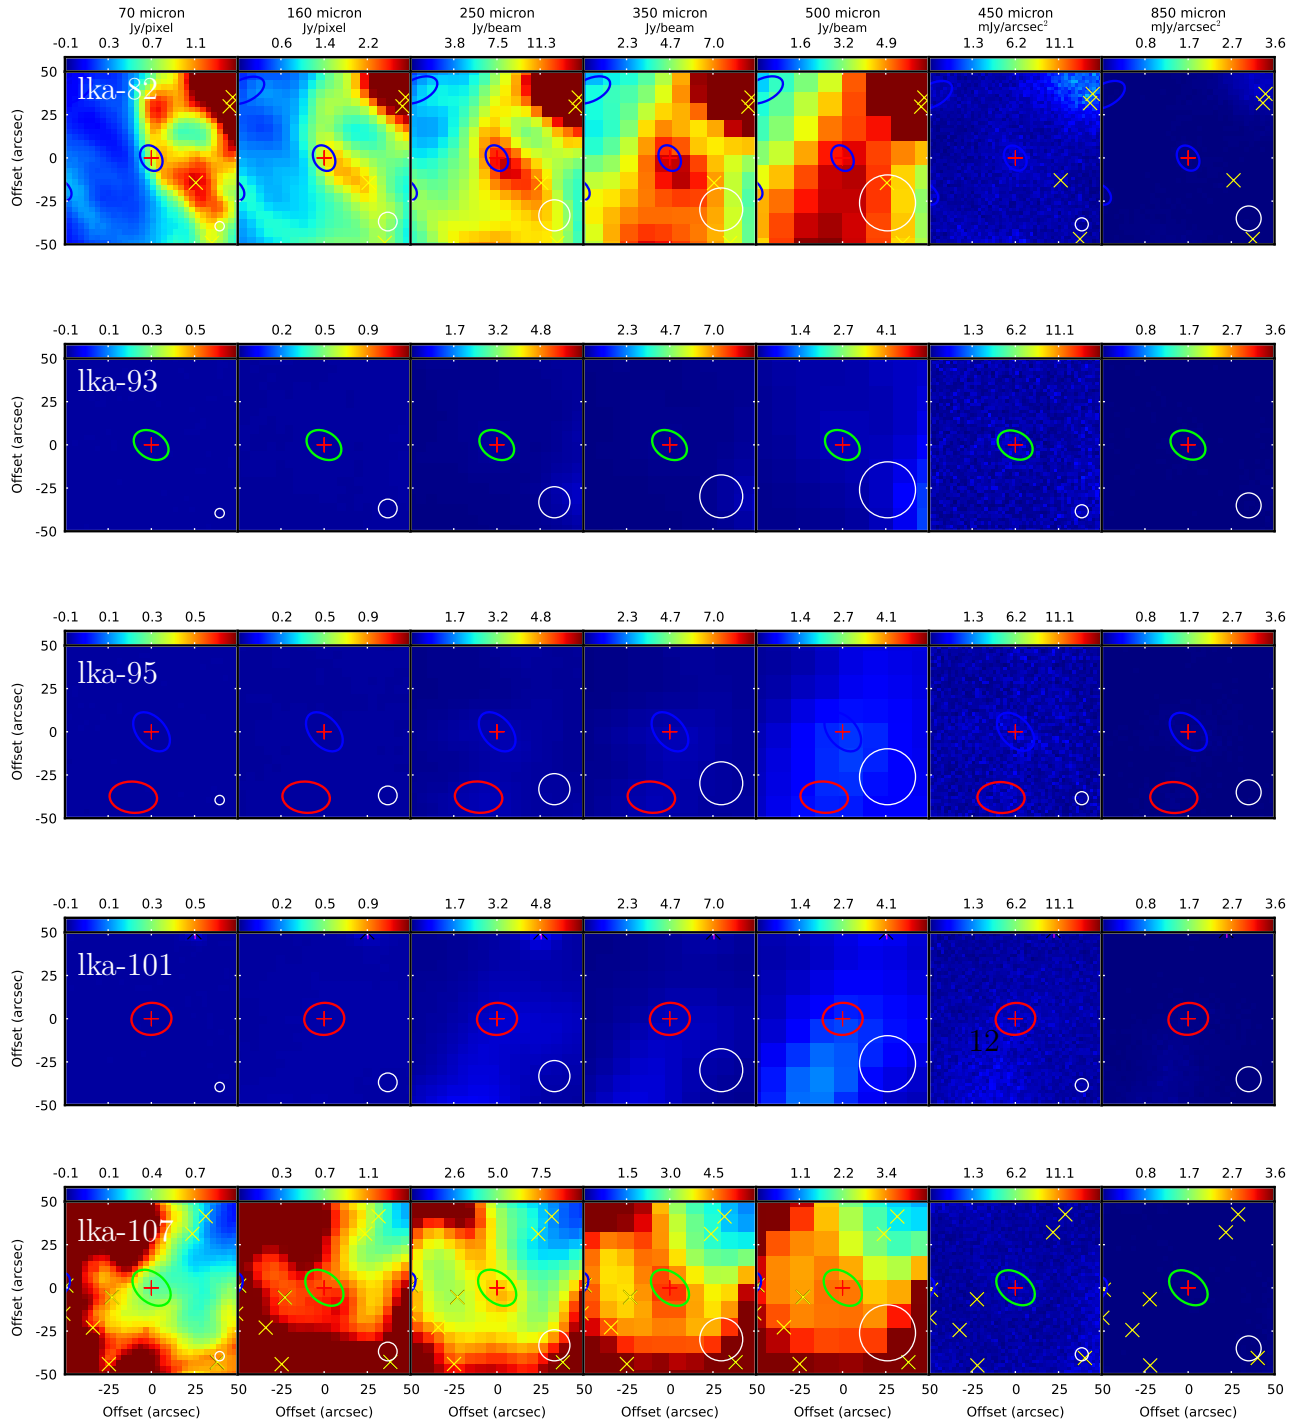

Figure 12:

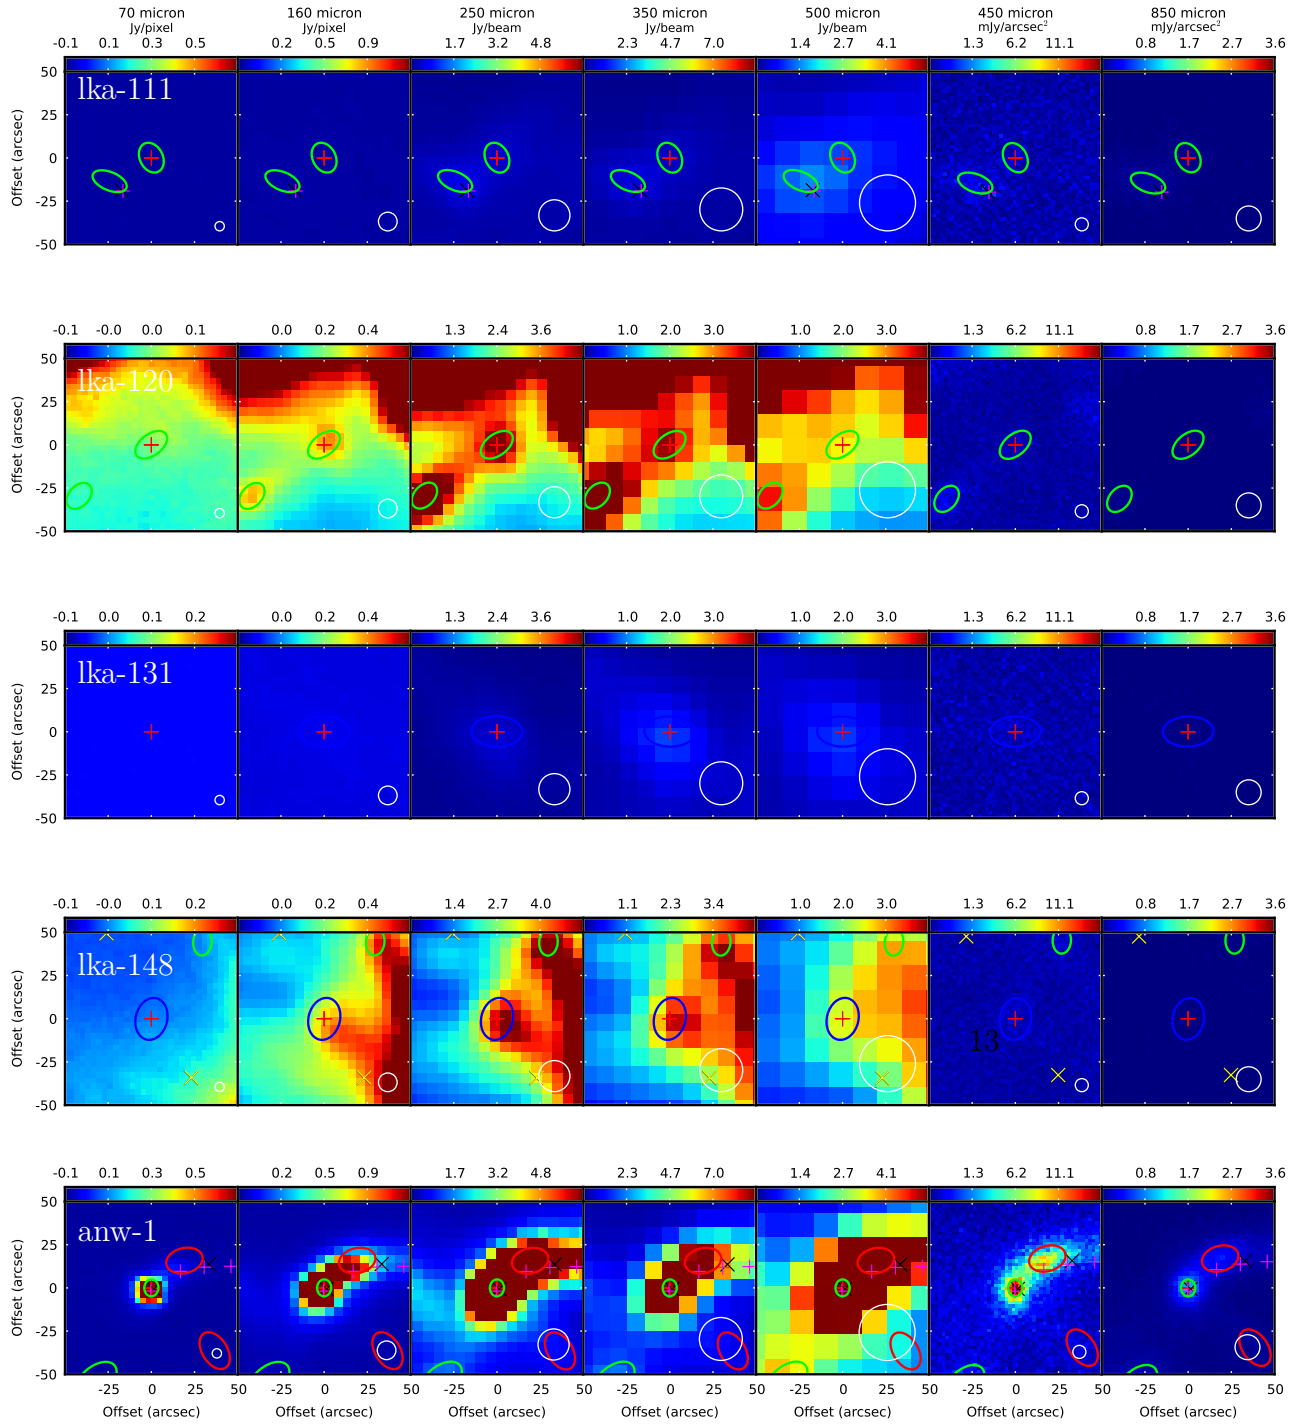

Figure 13:

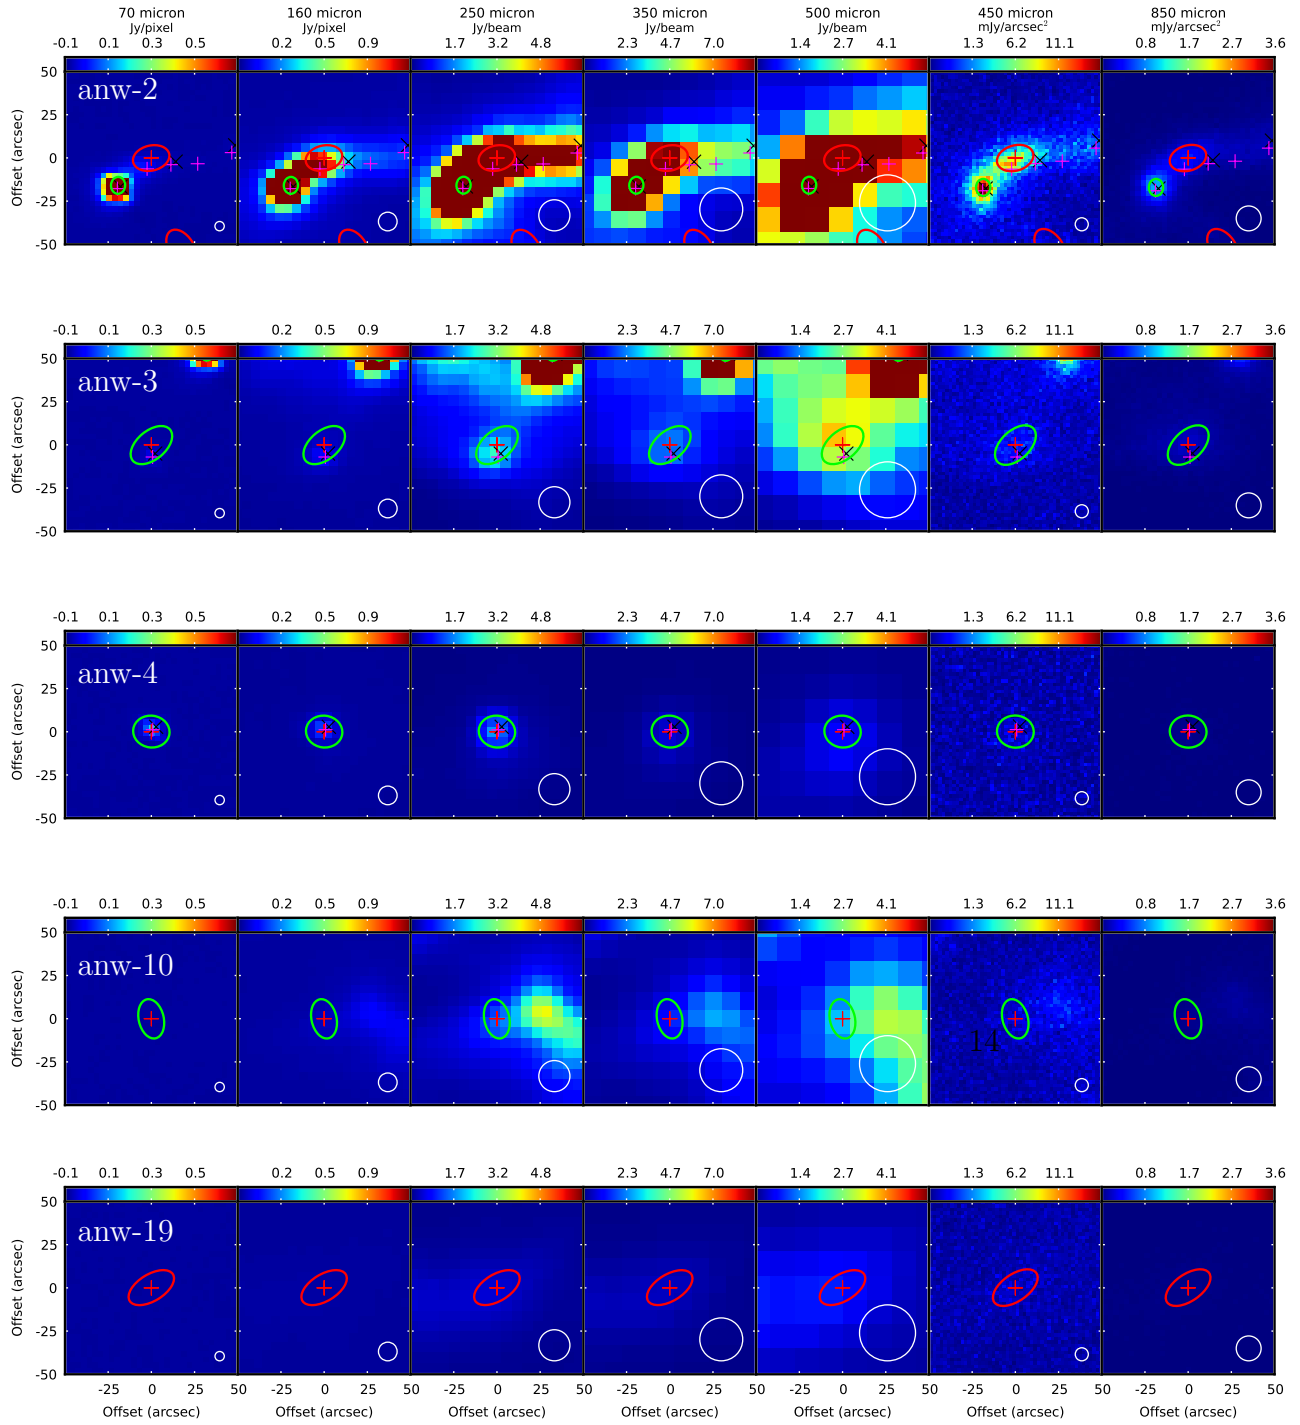

Figure 14:

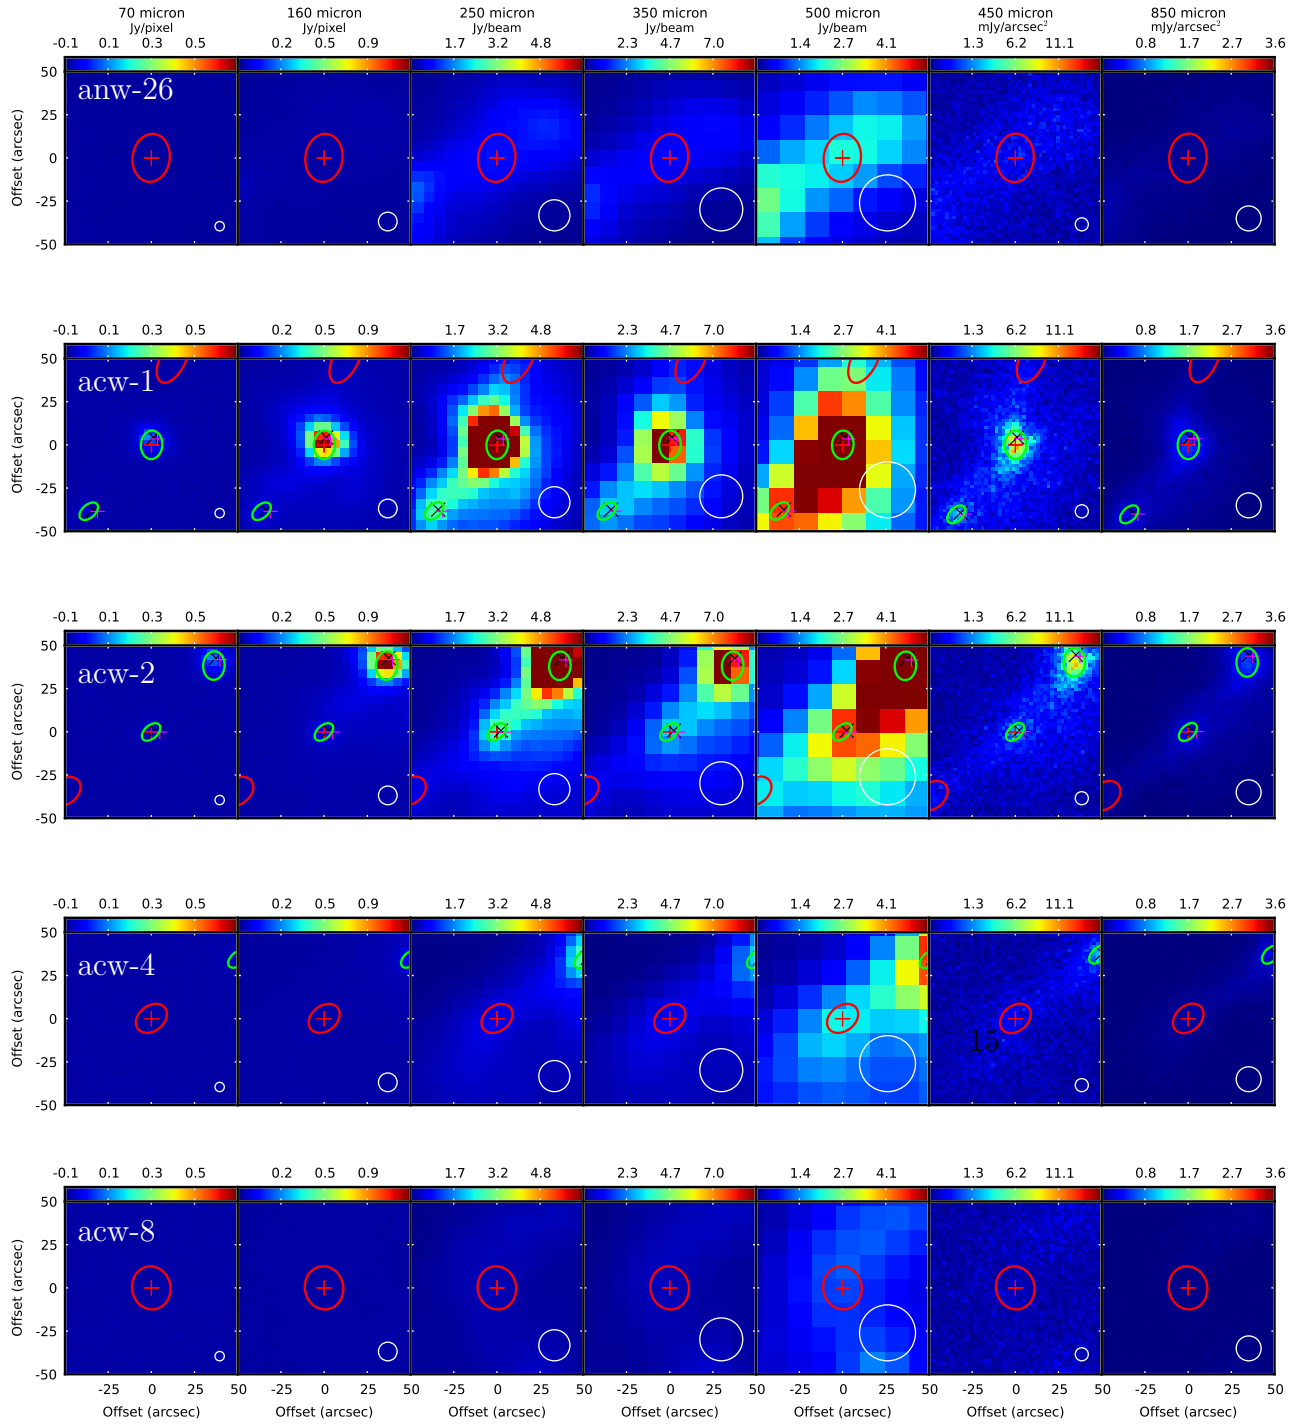

Figure 15:

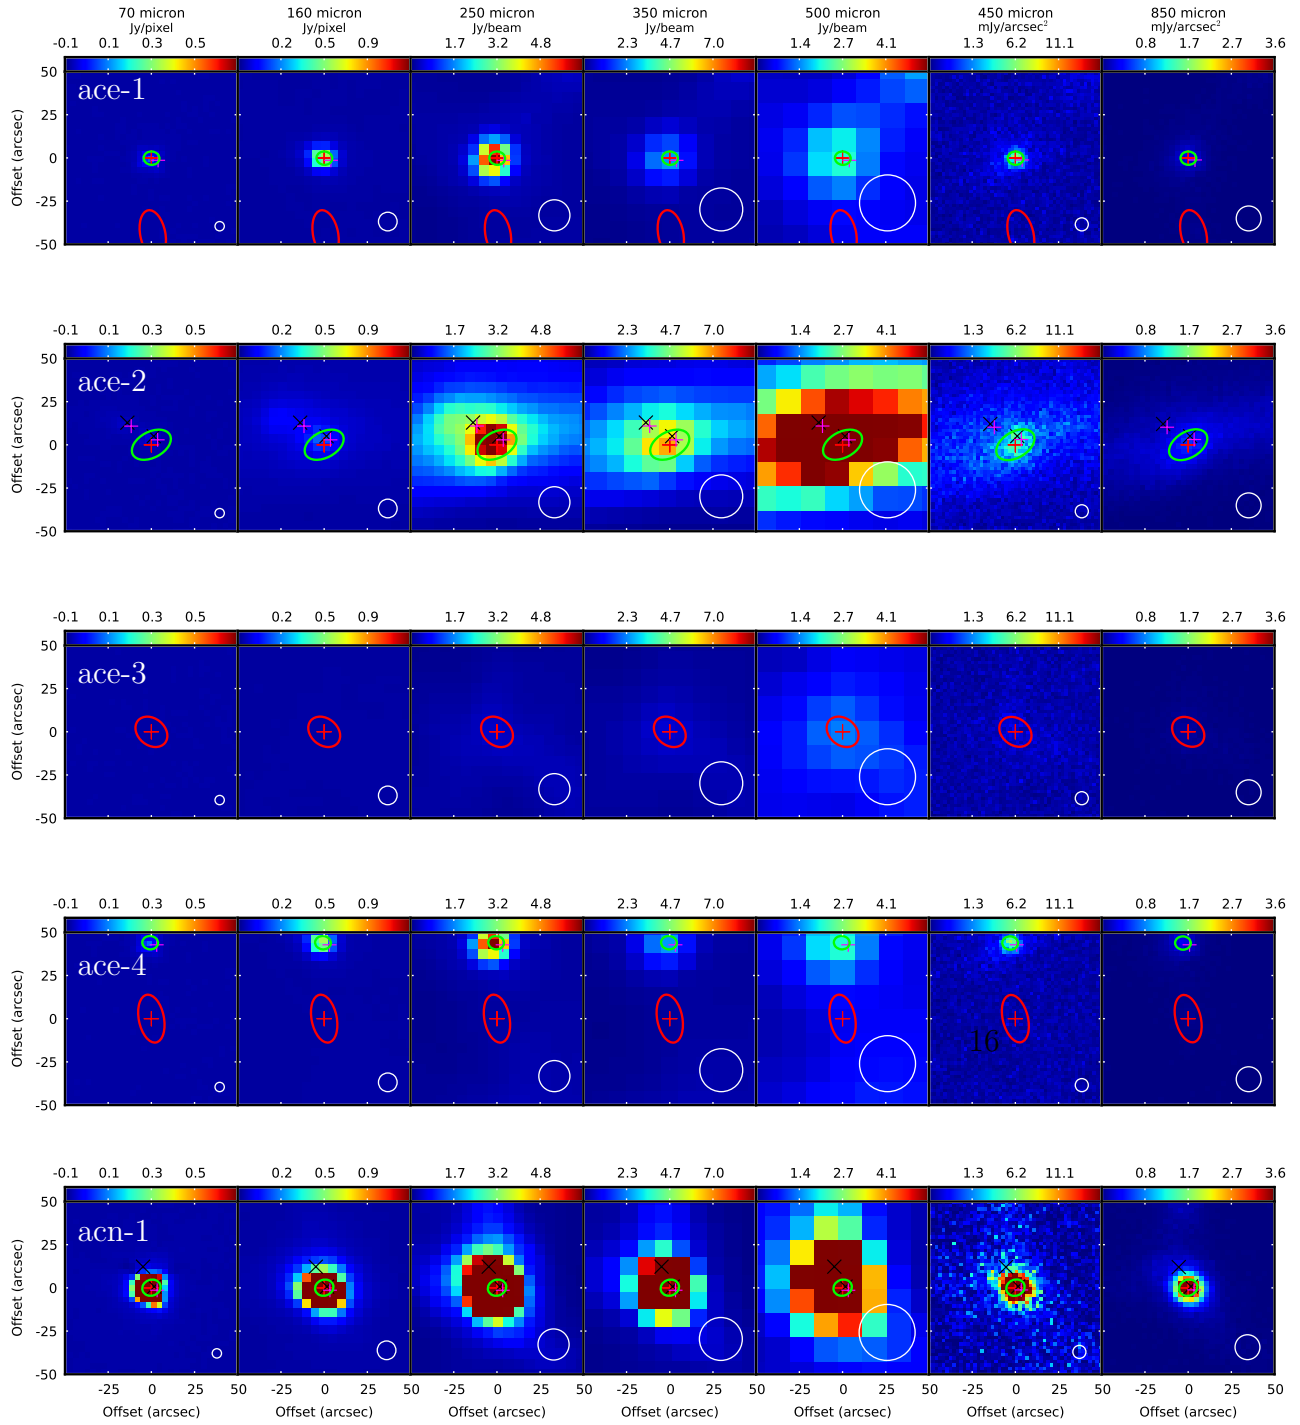

Figure 16:
